# Supplementary material for: Rhino: Deep Causal Temporal Relationship Learning With History-dependent Noise
Source: arXiv:2210.14706 source file (2022-10-26)
Supplement: Supplementary file 1 [file Additional_results.tex]

\section{Additional Results}
\label{app: Additional results}

\subsection{Additional synthetic experiments}
\label{subapp: additional synthetic experiments}

\subsection{Additional DREAM3 ROC Curve}

\subsection{Additional Netsim ROC Curve}
